# Supplementary material for: Towards Improving the Explainability of Text-based Information Retrieval with Knowledge Graphs
Source: arXiv:2301.06974 source file (2023-01-17)
Supplement: Supplementary file 1 [file appendix.tex]

\section{Appendix}
\label{appendix}
% \todo[]{Link to be inserted later}
Additional material, including source code for the experiments, data annotations are available at this (anonymized) link: \url{https://figshare.com/s/11012755a9cceab0d950}.
